# Supplementary material for: To Index or Not to Index: Optimizing Exact Maximum Inner Product Search
Source: arXiv:1706.01449 source file (2019-03-15)
Supplement: Supplementary file 1 [file appendix.tex]

\appendix
\normalsize

\begin{figure*}[ht!]
  \includegraphics[width=\textwidth]{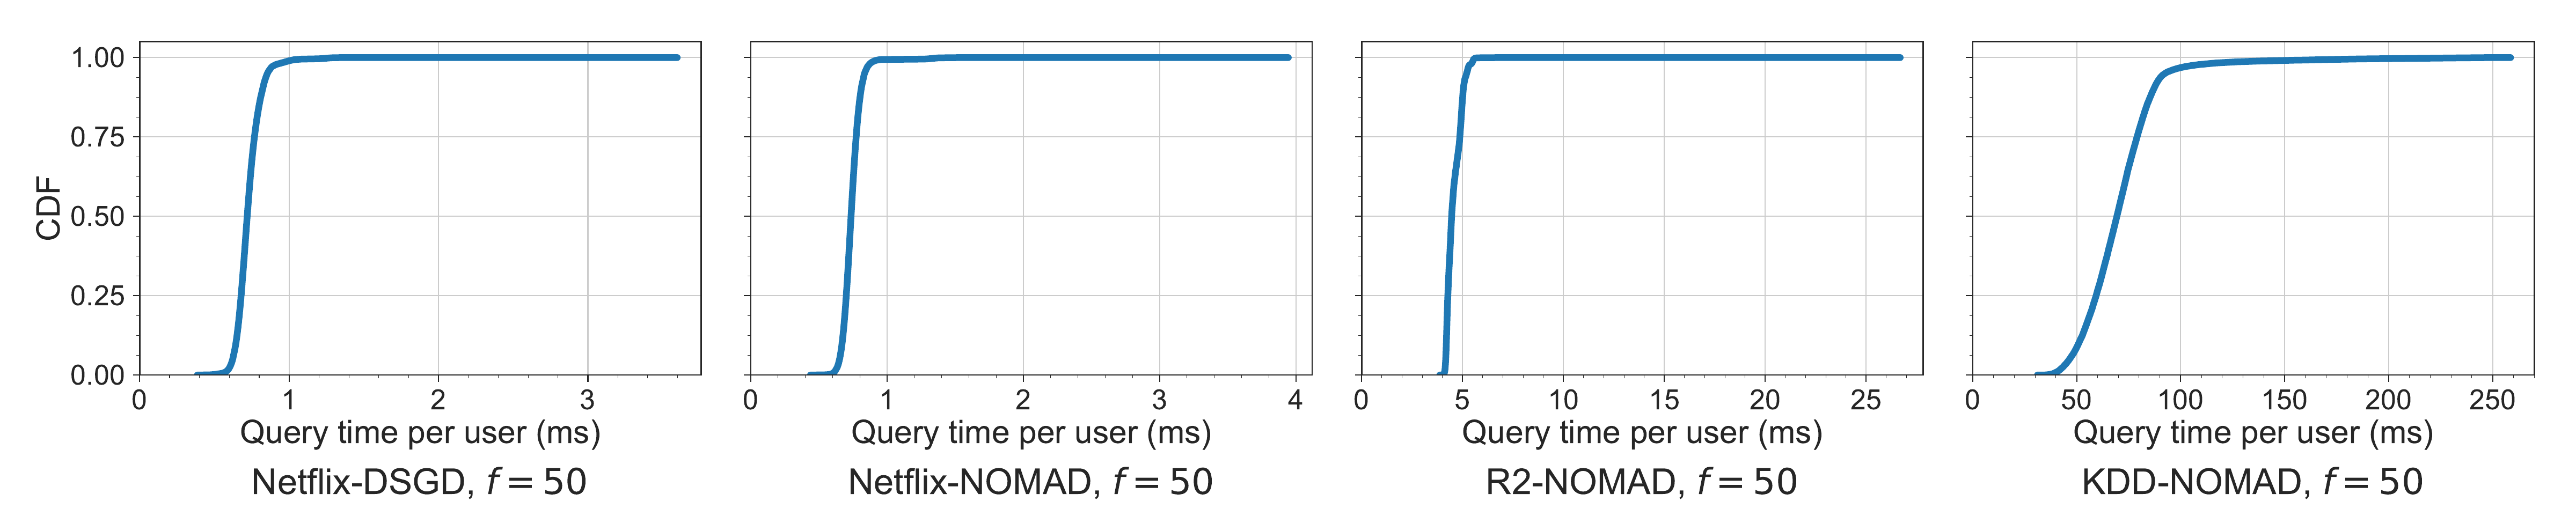}
  \caption{Distribution of point query times for $K=1$ using
    \simdexi. \simdex can also be used to serve point (i.e., online)
    queries for users with low latency if desired, although these point queries are not batched using work sharing.}
  \label{fig:query_time}
  \vspace{-1em}
\end{figure*}

\section{Training Parameters}
\label{sec:training_params}

For our benchmark experiments, we trained 12 models using the NOMAD toolkit~\cite{yun2014nomad}, as
described in Section~\ref{sec:evaluation}, tuning the regularization parameter
$\lambda$ using grid search. We report the best $\lambda$ setting found and the
corresponding test RMSE for these 12 models in
Table~\ref{table:training_params}.

\begin{table}[ht!]
\centering
\begin{tabular}{@{}llll@{}}
\toprule
Model                          & $f$ & $\lambda$ & Test RMSE \\ \midrule
\multirow{4}{*}{KDD-NOMAD}     & 10  & 1         & 26.0586   \\
                               & 25  & 0.001     & 25.7846   \\
                               & 50  & 1         & 26.2158   \\
                               & 100 & 1         & 26.2066   \\ \midrule
\multirow{4}{*}{Netflix-NOMAD} & 10  & 0.05      & 0.926713  \\
                               & 25  & 0.05      & 0.918437  \\
                               & 50  & 0.05      & 0.916493  \\
                               & 100 & 0.05      & 0.918999  \\ \midrule
\multirow{4}{*}{R2-NOMAD}      & 10  & 0.001     & 1.18179   \\
                               & 25  & 0.001     & 1.1707    \\
                               & 50  & 0.000001  & 1.17658   \\
                               & 100 & 0         & 1.20848   \\ \bottomrule
\end{tabular}
\caption{Optimal Regularization parameters for the corresponding models we trained, and the Test RMSE.}
\label{table:training_params}
\end{table}

\section{Additional Experimental Results}
\label{sec:additionalexp}
\label{sec:microbenchmarks}

To further understand the performance of \sbi, we perform multiple microbenchmarks that
demonstrate the source of its speedups. Specifically, we examine the
significance of tuning the number of clusters during the $k$-means step o
\simdexi's index construction and the importance of blocking for \simdexi's
high performance.

\begin{centering}
  \begin{figure*}[t!]
    \includegraphics[width=\textwidth]{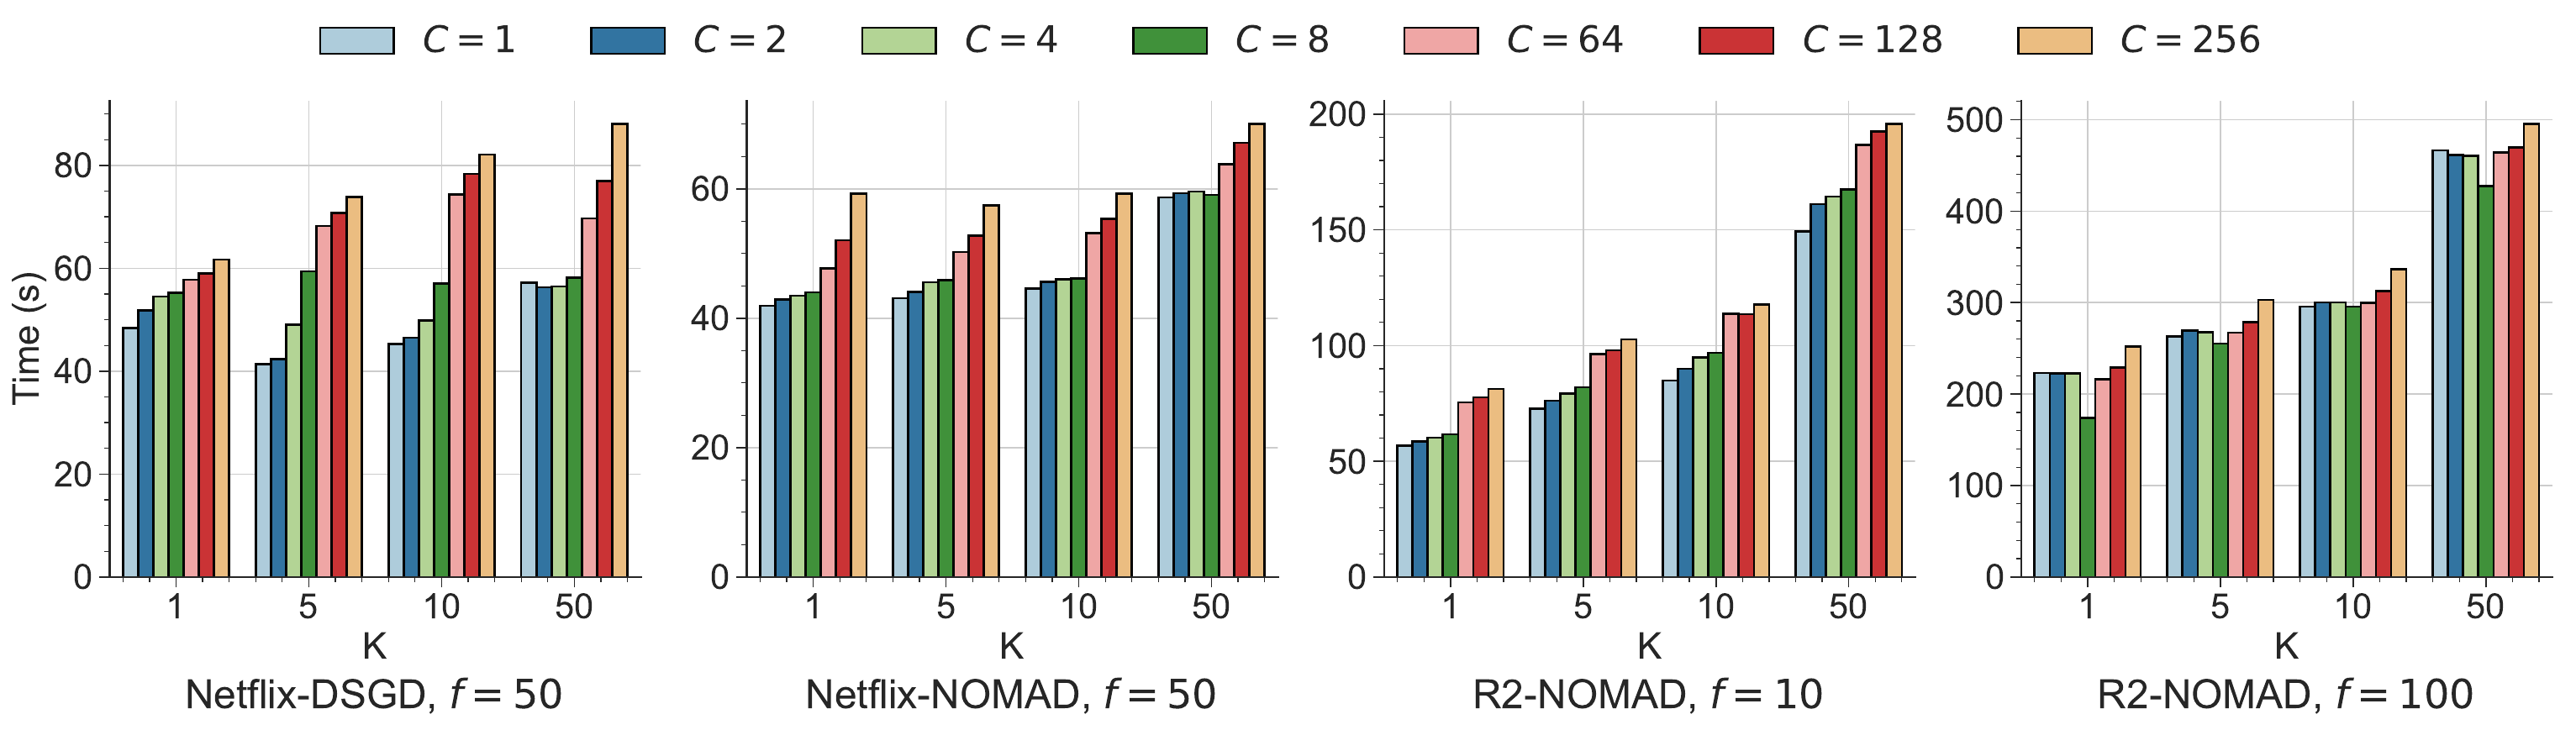}
    \caption{Runtime vs.~\# of clusters for \simdexi. A choice of
    $C=\{1,2,4\}$ typically delivers the best performance across our reference
    models.}
    \label{fig:runtime_num_clusters}
    \vspace{-1em}
  \end{figure*}
\end{centering}

\begin{centering}
  \begin{figure*}[t!]
    \includegraphics[width=\textwidth]{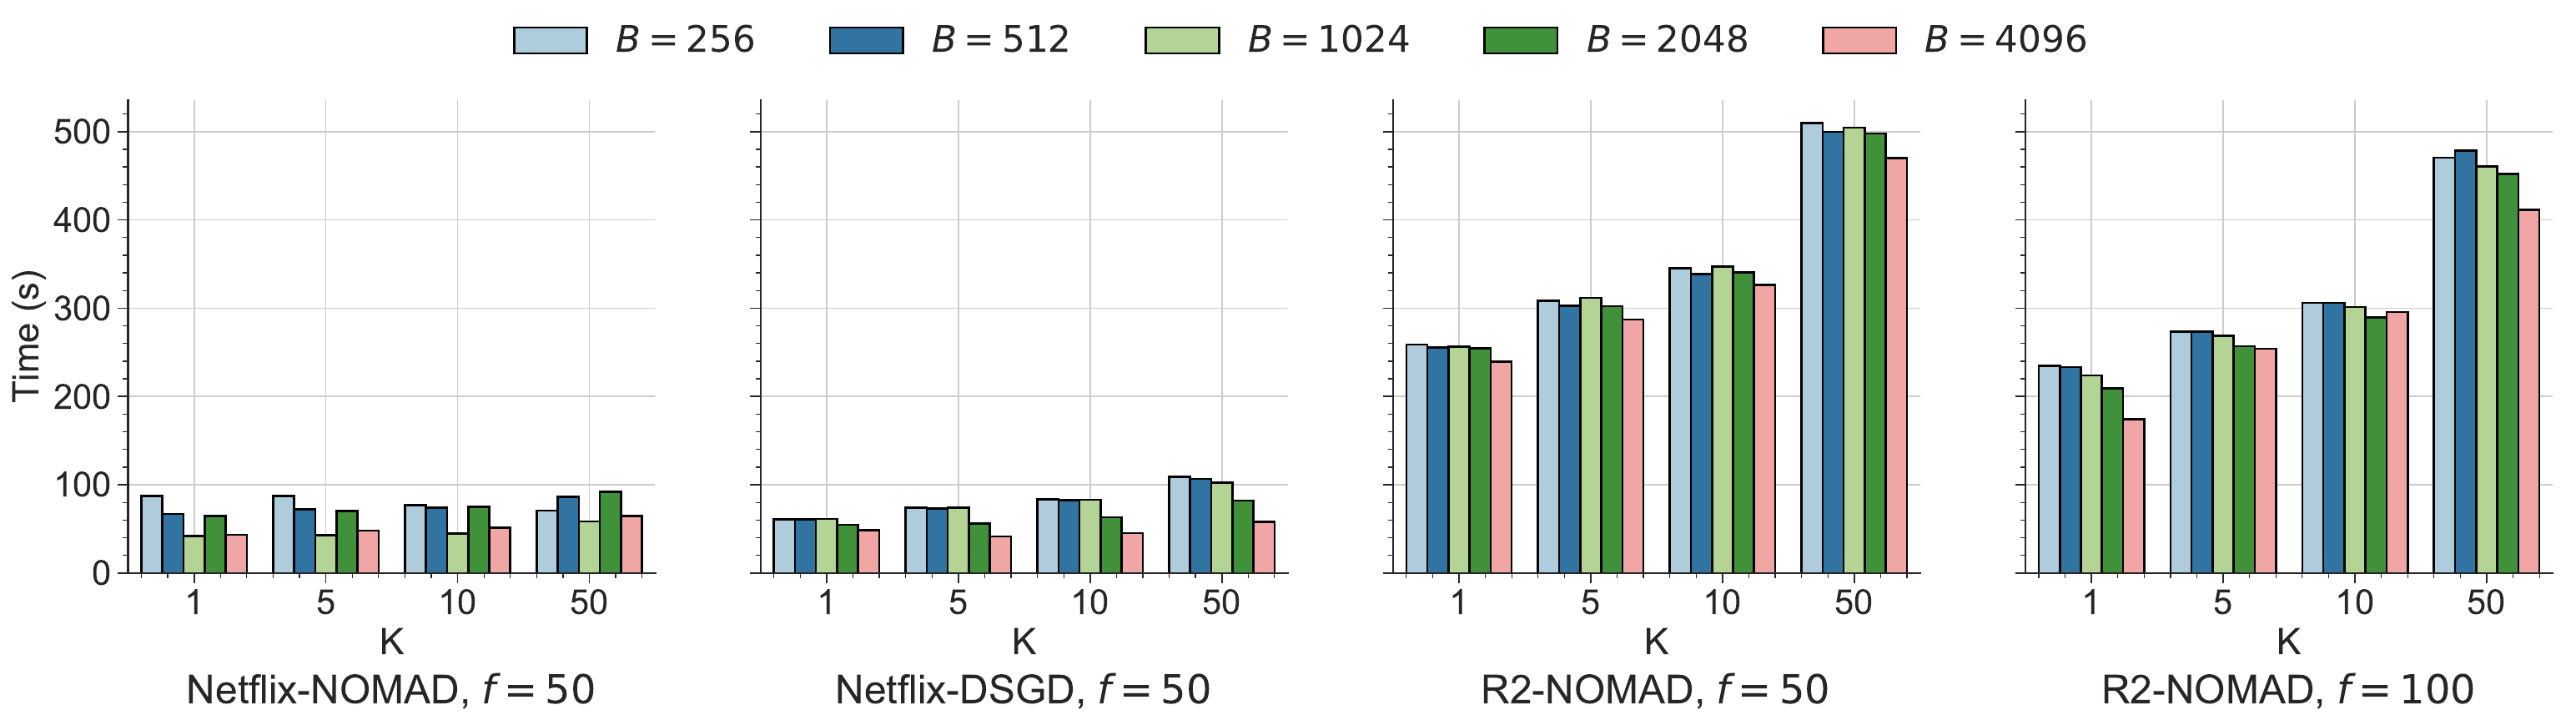}
    \caption{Runtime vs. $B$, the hardware blocking factor, for \simdexi. A choice of
    $B=\{1024,2048,4096\}$ typically delivers the best performance.}
    \label{fig:runtime_batch_size}
    \vspace{-1.5em}
  \end{figure*}
\end{centering}

\minihead{Clustering and blocking factor sensitivity analysis} To understand
the effect of \simdex's clustering and blocking on end-to-end runtime, we ran
two separate experiments in which we varied the number of clusters and blocking
factor in \simdex. Figure~\ref{fig:runtime_num_clusters} illustrates the
trade-off between clustering time and computation time for each dataset: more
clusters require more time to compute but subsequently reduce the computational
overhead of later steps, while fewer clusters require less time to compute but
increase the computational overhead of later steps. Clustering time increases
roughly proportionally to the number of clusters, while computational time
decreases in a dataset-dependent manner. Overall, we find that a small number
of clusters ($C=\{1,2,4\}$) performs well across the target models, including
those not depicted. Similarly, in our blocking factor experiment, we find that
small number of blocking factors ($B=\{1024,2048,4096\}$) performs well across
our target models; Figure~\ref{fig:runtime_batch_size} shows these results.
Given the relative robustness of these parameters to mild perturbations, we
believe that a small amount of tuning (if any) beyond this reasonable default
will perform well in practice.

\minihead{Per-User Point Queries} As noted in
Section~\ref{sec:background}, given the popularity of storing MF
predictions in low-latency online stores that are substantially more
computationally efficient than any online prediction strategy, we have
optimized \simdex for the batch setting. As we have discussed
in Section~\ref{sec:background}, \simdex is optimized for the batch
setting, where all users' recommendations are computed at once, as is
common in many deployments. However, if desired, \simdex can support
point queries (i.e., online queries, without pre-computing all users
and all items). Following index construction, \simdex can stop
processing and instead only compute user predictions on demand. The
cost of this strategy is that, unless multiple user requests from a
single cluster arrive at once, \simdex is unlikely to benefit from
work-sharing (but can still perform library-accelerated matrix-vector
multiply).

To
investigate the performance implications of this option, we measured
the latency of \simdex's index for point queries with
hardware-efficient work sharing disabled. Figure~\ref{fig:query_time}
depicts the results for single-user queries across several models; we
plot a CDF of the query latencies to show the distribution of runtime
performance for the users in the dataset. Following index
construction, for two Netflix models, \simdex's index averages 1.7 ms
per user, with median latency comparable to results reported by
FEXIPRO for this model. In contrast, the KDD and R2 models have more
items, resulting in query latencies from four to tens of
milliseconds. These latencies are lower than waiting to compute a
full, batched matrix multiply for all users but in turn incur a
throughput penalty as depicted in Figure~\ref{fig:factor_analysis}
because point queries do not benefit from work sharing unless batched.
